# Supplementary material for: RIPCN: A Road Impedance Principal Component Network for Probabilistic Traffic Flow Forecasting
Source: arXiv:2512.21685 source file (2025-12-25)
Supplement: Supplementary file 1 [file appendix_compute_cost.tex]

\setlength{\tabcolsep}{3pt}
\begin{table}[h]
\centering
\small
\caption{The GPU cost, training time, and inference time for different methods. The GPU cost is given in megabytes (MB), while the training time and inference time are expressed in seconds per batch (s/batch), with the batch size set to 12 and the number of samples is set to 10. The inference time for RIPCN includes the time for the mean predictor to generate the mean prediction and the time for uncertainty estimation.}
\label{gpu_time}
\arrayrulecolor{black}
\begin{tabular}{c|l|c c c}
\toprule
\textbf{Dataset} & \textbf{Method} & \textbf{GPU cost} & \textbf{Training time } & \textbf{Inference time} \\
\midrule
\multirow{8}{*}{PEMS03} 
& Latent ODE & 336 & 14522.38 & 357.02 \\
& DeepAR & 324 & 166.88 & 66729.01 \\
& MC Dropout & 2686 & 919.94 & 6220.72 \\
& STGNF & 20381 & 256.77 & 358.53 \\
& CSDI & 15236 & 581.09 & 30219.78 \\
& PriSTI & 8416 & 6623.72 & 38694.65 \\
& DiffSTG & 6568 & 440.13 & 35169.36 \\
& RIPCN & 11000 & 436.9 & 269.46+57.94 \\
\midrule
\multirow{8}{*}{PEMS04} 
& Latent ODE & 310 & 8032.08 & 923.73 \\
& DeepAR & 1748 & 110.21 & 1984.00 \\
& MC Dropout & 2348 & 638.05 & 4143.77 \\
& STGNF & 9303 & 215.73 & 827.74 \\
& CSDI & 14474 & 293.48 & 15700.41 \\
& PriSTI & 14178 & 3736.03 & 21343.61 \\
& DiffSTG & 5666 & 160.42 & 18453.13 \\
& RIPCN & 8214 & 228.91 & 148.22+28.12 \\
\midrule
\multirow{8}{*}{PEMS08} 
& Latent ODE & 274 & 4585.71 & 947.72 \\
& DeepAR & 1130 & 195.59 & 840.11 \\
& MC Dropout & 1378 & 501.15 & 2014.41 \\
& STGNF & 8199 & 142.12 & 238.85 \\
& CSDI & 8172 & 157.14 & 7817.96 \\
& PriSTI & 7970 & 2151.78 & 12037.01 \\
& DiffSTG & 3256 & 98.23 & 9752.73 \\
& RIPCN & 3952 & 117.84 & 50.13+16.77 \\
\midrule
\multirow{8}{*}{Seattle} 
& Latent ODE & 314 & 4487.24 & 475.45 \\
& DeepAR & 1846 & 74.07 & 145.81 \\
& MC Dropout & 2394 & 335.78 & 2548.25 \\
& STGNF & 17755 & 112.58 & 106.12 \\
& CSDI & 15334 & 177.28 & 9284.05 \\
& PriSTI & 14864 & 2082 & 11573.84 \\
& DiffSTG & 5972 & 88.41 & 9860.95 \\
& RIPCN & 8364 & 125.64 & 45.22+52.87 \\
\bottomrule
\end{tabular}
\end{table}
