# Supplementary material for: RIPCN: A Road Impedance Principal Component Network for Probabilistic Traffic Flow Forecasting
Source: arXiv:2512.21685 source file (2025-12-25)
Supplement: Supplementary file 2 [file appendix_mean_pre.tex]

\setlength{\tabcolsep}{3pt}
\begin{table}[ht]
\centering
\small
\caption{The performance of RIPCN based on different mean predictors.}
\label{maen_pred}
\arrayrulecolor{black}
\begin{tabular}{c|l|c c c c c}
\toprule
\textbf{Dataset} & \textbf{Method} & \textbf{MAE} & \textbf{RMSE} & \textbf{MAPE} & \textbf{CRPS} & \textbf{MIS} \\
\midrule
\multirow{6}{*}{PEMS03} 
& DiffSTG & 18.47 & 32.27 & 28.03 & 0.0997 & \underline{215.97} \\
& RIPCN(DiffSTG) & 15.99 & 27.18 & 17.71 & 0.1043 & 217.92 \\
& FC\_LSTM & 19.82 & 30.42 & 18.82 & / & / \\
& RIPCN(FC\_LSTM) & 17.31 & 29.39 & 18.32 & 0.1054 & 231.61 \\
& STGCN & 22.62 & 36.11 & 27.48 & / & / \\
& RIPCN(STGCN) & 16.35 & 27.95 & 21.49 & 0.1169 & 232.47 \\
& ASTGNN & 16.51 & 27.43 & \underline{16.05} & / & / \\
& RIPCN(ASTGNN) & 16.46 & 27.19 & 16.80 &\underline{ 0.0807} & \textbf{172.17} \\
& PDFormer & \underline{15.46} & \underline{26.14} & 16.26 & / & / \\
& RIPCN(PDFormer) & \textbf{15.28} & \textbf{26.05} & \textbf{12.07} & \textbf{0.0778} & 221.34 \\
\midrule
\multirow{6}{*}{PEMS04} 
& DiffSTG & 21.90 & 33.99 & 16.54 & 0.0779 & 257.85 \\
& RIPCN(DiffSTG) & 20.24 & 32.83 & 14.15 & 0.0771 & 258.50 \\
& FC\_LSTM & 24.59 & 39.60 & 17.42 & / & / \\
& RIPCN(FC\_LSTM) & 20.91 & 33.91 & 14.38 & 0.0815 & 287.49 \\
& STGCN & 24.51 & 42.33 & 20.28 & / & / \\
& RIPCN(STGCN) & 20.91 & 33.33 & 15.86 & 0.0820 & 271.13 \\
& ASTGNN & \underline{18.69} & 31.23 & 12.31 & / & / \\
& RIPCN(ASTGNN) & \textbf{18.60} & 30.94 & \underline{12.27} & \underline{0.0721} & \underline{247.71} \\
& PDFormer & 19.05 &  \underline{30.76} & 12.87 & / & / \\
& RIPCN(PDFormer) & 19.03 & \textbf{30.19} & \textbf{11.06} & \textbf{0.0701} & \textbf{219.98} \\
\midrule
\multirow{6}{*}{PEMS08} 
& DiffSTG & 17.74 & 27.16 & 11.11 & 0.0607 & 215.96 \\
& RIPCN(DiffSTG) & 16.52 & 25.53 & 10.92 & 0.0598 & 212.19 \\
& FC\_LSTM & 26.19 & 44.95 & 14.09 & / & / \\
& RIPCN(FC\_LSTM) & 18.29 & 28.49 & 11.99 & 0.1106 & 289.27 \\
& STGCN & 23.44 & 33.44 & 16.87 & / & / \\
& RIPCN(STGCN) & 17.79 & 27.09 & 12.67 & 0.0657 & 234.70 \\
& ASTGNN & \underline{15.12} & 24.45 & 9.62 & / & / \\
& RIPCN(ASTGNN) & \textbf{15.04} & \textbf{24.30} & \underline{9.59} & \textbf{0.0563} & \textbf{203.36} \\
& PDFormer & 15.23 & 24.34 & 9.77 & / & / \\
& RIPCN(PDFormer) & 15.14 & \underline{23.76} & \textbf{9.27} & \underline{0.0565} & \underline{206.91} \\
\midrule
\multirow{6}{*}{Seattle} 
& DiffSTG & 127.05 & 203.83 & 27.47 & 0.1206 & 1761.73 \\
& RIPCN(DiffSTG) & 119.98 & 194.31 & 25.08 & 0.1244 & \underline{1353.14} \\
& FC\_LSTM & 127.04 & 199.80 & 25.29 & / & / \\
& RIPCN(FC\_LSTM) & 121.50 & 185.79 & 23.24 & 0.1538 & 1492.44 \\
& STGCN & 128.00 & 193.76 & 28.05 & / & / \\
& RIPCN(STGCN) & 123.74 & 185.82 & 27.56 & 0.1920 & 1678.51 \\
& ASTGNN & 100.79 & 172.92 & \textbf{18.95} & / & / \\
& RIPCN(ASTGNN) & \underline{98.89} & 165.97 & 19.06 & \underline{0.1048} & 1397.13 \\
& PDFormer & 102.17 & \underline{164.39} & 27.15 & / & / \\
& RIPCN(PDFormer) & \textbf{94.97} & \textbf{147.74} & \underline{18.98} & \textbf{0.0955} & \textbf{1297.79} \\
\bottomrule
\end{tabular}
\end{table}
